# Supplementary material for: Theoretical Understandings of Product Embedding for E-commerce Machine Learning
Source: arXiv:2102.12029 source file (2021-02-24)
Supplement: Supplementary file 1 [file appendix.tex]

The proofs in the appendix are mostly technical. Due to the eight-page space limit (including appendix), here we only list the key steps and omit the tedious parts \footnote{We will provide the readers an online material containing the detailed proof after the double-blind review}. 

\textbf{Proof for Claim \ref{claim:sdr}}.
% \begin{proof}
The first-order necessary condition for the global optimal (without dimension constraint) $\Zbf^*$, $\tilde{\Zbf^*}$ is given by $\nabla_{\zbf_i} \ell(\Dcal) = 0$, $\nabla_{\tilde{\zbf}_i} \ell(\Dcal) = 0$.
According to (\ref{eqn:grad-sgns}), it implies that $\langle \zbf_i^*, \tilde{\zbf}_i^* \rangle = R_{i,j}$ for all $i,j \in \Ical$. Note that minimizing $\ell(\Dcal)$ is equivalent to finding 
$
\arg\min_{\Zbf, \tilde{\Zbf} \in \Rbb^d} \big\{\ell(\Dcal) -  \min_{\Zbf, \tilde{\Zbf}}\ell(\Dcal) \big\},
$
where by the above argument the second term is given by:\\
$
\sum_{i, j \in \Ical} N_{i,j}(\Dcal) \log \sigma(R_{i,j}) + \frac{k}{n} N_i(\Dcal) N_j(\Dcal) \log \sigma(-R_{i,j}).
$
By rearranging terms and extracting the factor of $n(k+1)$ to the outside, we have:
\begin{equation}
\begin{split}
    & n(k+1)\big(\ell(\Dcal) -  \min_{\Zbf, \tilde{\Zbf}}\ell(\Dcal) \big) = \sum_{i,j \in \Ical} \Big\{\frac{1}{k}p_{i,j}(\Dcal)\log\frac{\sigma(R_{i,j})}{\sigma(\zbf_i^{\intercal}\zbf_j)} + \\
    & \qquad \qquad (1-\frac{1}{k})p_i(\Dcal)p_j(\Dcal)\log\frac{\sigma(-R_{i,j})}{\sigma(-\zbf_i^{\intercal}\zbf_j)} \Big\} \\
    & = \sum_{i,j \in \Ical} \Big\{\frac{1}{k}p_{i,j}(\Dcal)\log\frac{p\big(O=1|(i,j);R\big)}{q\big(O=1|(i,j);\zbf_i,\tilde{\zbf}_j\big)} + \\
    & \qquad \qquad (1-\frac{1}{k})p_i(\Dcal)p_j(\Dcal)\log\frac{p\big(O=0|(i,j);R\big)}{q\big(O=0|(i,j);\zbf_i,\tilde{\zbf}_j\big)} \Big\} \\
    & = \sum_{\substack{\alpha \in \{0,1\} \\ (i,j)\in \Dcal}}p\big(O=\alpha, (i,j)\big)\log \log\frac{p\big(O=\alpha|(i,j);R\big)}{q\big(O=\alpha|(i,j);\zbf_i,\tilde{\zbf}_j\big)} \Big\} \\
    & = D_{KL}\Big( q\big(O \, \big| \, \Dcal;\, \Zbf,\tilde{\Zbf}\big) \, \big\| \, p\big(O \, \big| \, \Dcal;\, R\big) \Big).
\end{split}
\end{equation}
Hence we obtain the desired result.
% \end{proof}

\textbf{Proof for Lemma \ref{lemma:CI}}
% \begin{proof}
We use the Cramer-Chernoff method. Let $u_{i,j} = \Ebb[N_{i}(\Dcal)] \cdot \Ebb[N_{j}(\Dcal)]/n^2$. For some $\lambda > 0$, we have:
\begin{equation*}
\begin{split}
    & p\Big(\frac{N_{i,j}(\Dcal)}{n} \geq  u_{i,j} + \epsilon \Big) = p\Big(\exp\Big(\lambda \sum_{i,j} \ind[j \in \Ncal(i)] -  u_{i,j} \Big) \geq \exp(\lambda n \epsilon)  \Big) \\ 
    & \leq \frac{\Ebb\big[ \exp\Big(\lambda \sum_{i,j} \ind[j \in \Ncal(i)] - u_{i,j} \big]}{\exp(\lambda n \epsilon)} \\
    & = \big(u_{i,j}\exp \big(\lambda(1-u_{i,j}-\epsilon) \big) + (1-u_{i,j})\exp\big( -\lambda(u_{i,j}+\epsilon) \big) \big)^n.
\end{split}
\end{equation*}
The expression is minimized by $\lambda^* = \log \frac{(u_{i,j}+\epsilon)(1-u_{i,j})}{u_{i,j}(1-u_{i,j}-\epsilon)}$. We plug $\lambda^*$ back and obtain:
\[ 
p\Big(\frac{N_{i,j}(\Dcal)}{n} \geq  u_{i,j} + \epsilon \Big) = \exp\big(-nD_{KL}(u_{i,j} + \epsilon \| u_{i,j})  \big).
\]
After a change of variable, we obtain the desired tail bound. To obtain the confidence set, simply notice that $D_{KL}(\cdot \| u_{i,j})$ is decreasing on $[0,u_{i,j}]$, so for $0\leq\beta \leq D_{KL}(0\|u_{i,j})$, we have $\big\{D_{KL}\big(\frac{N_{i,j}(\Dcal)}{n} \| u_{i,j}\big) \geq \beta, \frac{N_{i,j}(\Dcal)}{n} \leq u_{i,j}\big\} = \big\{\frac{N_{i,j}(\Dcal)}{n} \leq u_{i,j} - \alpha\big\}$, where $\alpha$ is the unique solution to $D_{KL}\big(u_{i,j} - \alpha)\| u_{i,j}\big) = \beta$ on $[0,u_{i,j}]$. Hence, \\ $p\Big(D_{KL}\big(\frac{N_{i,j}(\Dcal)}{n} \| u_{i,j}\big) \geq \beta, \frac{N_{i,j}(\Dcal)}{n} \leq u_{i,j} \Big) \leq \exp(-n\beta)$. The rest of derivation follows by simple algebra.
% \end{proof}

\textbf{Proof for Claim \ref{claim:higher-order}}.
% \begin{proof}
Define shorthand $\vec{I} = \{i_1,\ldots,i_k\}$ and $p(i|j) = p\big(\ind [j \in \Ncal(i)])$. 
\begin{equation*}
\begin{split}
& D_{KL}\Big(p\big(\ind\big[i \in \Ncal(\{i_1,\ldots,i_k\})\big]\big) \,\big\|\, p\big(\ind[i \in \Ncal(i^*)]\big)  \Big) \\
& = \sum_{k}p(k|\vec{I}) \Big( \log \frac{p(\vec{I})}{\prod_{i \in \vec{I}}p(i)} - \log \frac{p(\vec{I}|k)}{\prod_{i\in \vec{I}}p(i|k)} \\
    &\quad  + \log \frac{p(i^* | k)}{p(i^*)} - \log \prod_{i\in \vec{I}}\frac{p(i|k)}{p(i)} \Big), \\
    % &= \sum_{k}p(k|\vec{I}) \Big( \log \frac{p(\vec{I})}{\prod_{j \in \vec{I}}p(j)} - \log \frac{p(\vec{I}|k)}{\prod_{j\in \xbf}p(j|k)} + \Rbf_{i^*,k} - \sum_{i \in \vec{I}}\Rbf_{i,k} \Big) \\
    % & = \Ebb_{i|\vec{I}}\Big[ \log \frac{p(\vec{I})}{\prod_{j \in \vec{I}}p(j)} - \log \frac{p(\vec{I}|i)}{\prod_{j\in \xbf}p(j|i)} - \sum_{i \in \vec{I}}\Rbf_{i,i} \Big] + \Ebb_{i | \vec{I}} \big[\Rbf_{i^*,i} \big]
\end{split}
\end{equation*}
which is given by: $\sum_{k}p(k|\vec{I}) \Big( \log \frac{p(\vec{I})}{\prod_{j \in \vec{I}}p(j)} - \log \frac{p(\vec{I}|k)}{\prod_{j\in \xbf}p(j|k)} + \Rbf_{i^*,k} - \sum_{i \in \vec{I}}\Rbf_{i,k} \Big)$, and leads to:
\[ 
\Ebb_{i|\vec{I}}\Big[ \log \frac{p(\vec{I})}{\prod_{j \in \vec{I}}p(j)} - \log \frac{p(\vec{I}|i)}{\prod_{j\in \xbf}p(j|i)} - \sum_{i \in \vec{I}}\Rbf_{i,i} \Big] + \Ebb_{i | \vec{I}} \big[\Rbf_{i^*,i} \big].
\]
Notice that the first term is independent of $i^*$, so when 
\[ 
D_{KL} \big(p(I | \vec{I}) || p(I | i^*)\big) \leq D_{KL} \big(p(j | \vec{I}) || p(I | j)\big)
\]
$\forall j \in \Ical$, we have: $\Ebb_{I | \vec{I}} \big[\Rbf_{i^*,I} - \Rbf_{j,I}  \big] \geq 0, \forall j \in \Ical.$ Each step is invertible, so we obtain the desired result.
% \end{proof}

\textbf{Proof for Claim \ref{claim:functional}}.
The key step for proving Claim \ref{claim:functional} and recover the formalized statement is to recognize:
\begin{equation*}
\label{eqn:appendix1}
\begin{split}
   & \Rbf_{i^*,k} - \Rbf_{i,k} \\
   & = \log \frac{p(k|i^*)}{p(k|i)} + \log \prod_{q^{+} \in \Dcal_r^{+}}\frac{p(k|q^+)}{p(k|q^+)} + \log \prod_{q^- \in \Dcal_r^{-}}\frac{p(k|q^-)}{p(k|q^-} 
\end{split}
\end{equation*}
by splitting $\Dcal_r$ into $\Dcal_r^{+} \cup \Dcal_r^{-}$, where $\Dcal_r^{+}=\{i \, |\,  \exists j \in \Ical \, s.t. \, (i,j) \in \Dcal_r\}$ and $\Dcal_r^{+}=\{j \, |\,  \exists i \in \Ical \, s.t. \, (i,j) \in \Dcal_r\}$. The rest of the proof are simply algebraic manipulation and regrouping terms.  

\textbf{Proof for Theorem \ref{thm:generalization}}
% \begin{proof}
Define $\theta_1^* = \arg\min_{\theta}\sum_{i=1}^{|\Ical|}\phi(\zbf_i^{\intercal}\theta, \ybf_i)$ and $\hat{y}(\Zbf)=\Zbf^{\intercal}\theta_1^*$. The $\theta_2^*$ and $\hat{y}(\Xbf)$ are defined similarly. Let $\Phi(\hat{\ybf}, \ybf) = \frac{1}{n}\sum_{i=1}^{|\Ical|}\phi\big(\hat{\ybf}_i,\ybf_i\big)$ be the average training loss and similarly, $\Phi\big(\hat{\ybf}, \Ubf(X)^{\intercal}\thetabf_0\big)$ is the average test loss. Note that $\Phi(\cdot,\cdot)$ is $\frac{L}{\sqrt{n}}$-Lipschitz in both arguments. By the definition of $\phi$ as a loss function, $\Ubf(X)^{\intercal}\thetabf_0 = \arg\min_{\hat{\ybf}}\Phi\big(\hat{\ybf},\Ubf(X)^{\intercal}\thetabf_0\big)$, so:
\begin{equation}
\label{eqn:thm-1}
    \Lcal(\Xbf) = \Ebb_{\epsilon}\Big[\Phi\big(\hat{\ybf}(\Xbf), \Ubf(X)^{\intercal}\thetabf_0\big)\Big] \geq \Phi\big(\Ubf(X)^{\intercal}\thetabf_0,\Ubf(X)^{\intercal}\thetabf_0\big).
\end{equation}
On the other hand, for all $\theta_1$ we have:
\begin{equation}
\label{eqn:thm-2}
\begin{split}
\Lcal(\Zbf) &= \Ebb_{\epsilon}\big[ \Phi\big(\hat{\ybf}(\Xbf)\big), \Ubf(X)^{\intercal}\thetabf_0 \big] \\ 
& \leq \Ebb_{\epsilon}\Big[\Phi\big(\Ubf(\Zbf)^{\intercal}\theta_1^*, \ybf\big) + \frac{L}{\sqrt{n}} \big\| \ybf - \Ubf(X)^{\intercal}\thetabf_0 \big\| \Big] \\ 
& \leq \Ebb_{\epsilon} \Big[\Phi\big(\Ubf(\Zbf)^{\intercal}\theta_1, \Ubf(X)^{\intercal}\thetabf_0\big) + \frac{L}{\sqrt{n}}\big\|\Ubf(X)^{\intercal}\thetabf_0 - y\big\| \Big] + \Ebb_{\epsilon}\big[\frac{L}{\sqrt{n}}\|\epsilonbf\|   \big] \\ 
& \leq \Phi\big(\Ubf(\Zbf)^{\intercal}\theta_1, \Ubf(X)^{\intercal}\thetabf_0\big) + 2L\sigma,
\end{split}
\end{equation}
where we use the $\frac{L}{\sqrt{n}}$-Lipschitz of $\Phi$ and the definition of $\theta_1^*$. Let $\ybf_0 = \Ubf(X)^{\intercal}\thetabf_0$. Combining (\ref{eqn:thm-1}) and (\ref{eqn:thm-2}), we have:
\begin{equation}
\label{eqn:thm-3}
\begin{split}
\Ebb \big[\Lcal(\Zbf) -  \Lcal(\Xbf) \big] & \leq \Ebb\Big[\Phi\big(\Zbf^{\intercal}\theta_1, \ybf_0\big) + 2L\sigma -  \Phi\big(\ybf_0,\ybf_0\big) \Big] \\ 
& \leq \Ebb\Big[\frac{L}{\sqrt{n}} \big\|\Zbf^{\intercal}\theta_1 - \ybf_0  \big\| + 2L\sigma \Big].
\end{split}
\end{equation}
Notice that the least-square term $\big\|\Zbf^{\intercal}\theta_1 - \ybf_0 \big\|$ is bounded by: \\ $\sqrt{\|\ybf_0\|^2 - \big\|\Ubf(\Zbf)^{\intercal}\ybf_0\big\|^2}$ by textbook derivation, so we further have:
\begin{equation}
\Ebb \big[\Lcal(\Zbf) -  \Lcal(\Xbf) \big]  \leq \frac{L}{\sqrt{n}}\sqrt{\Ebb\Big[\|\ybf_0\|^2 - \big\|\Ubf(\Zbf)^{\intercal}\ybf_0\big\|^2 \Big]} + 2L\sigma,
\end{equation}
using the Jensen's inequality. Finally, using the definitions and simple algebra, we have: $\Ebb\big[\|\ybf_0\|^2  \big] = tr(\Sigma)$ and $\Ebb\big[ \big\|\Ubf(\Zbf)^{\intercal}\ybf_0\big\|^2 \big] \geq d\underline{\lambda(\Sigma)}\big\|\Ubf(X)^{\intercal}\Ubf(Z)\big\|_F^2$, and thus the desired result.
% \end{proof}
